# Supplementary material for: Is Big Data Performance Reproducible in Modern Cloud Networks?
Source: arXiv:1912.09256 source file (2019-12-19)
Supplement: Supplementary file 1 [file repro_appendix.tex]

reproducibility appendix:

Summarize the experiments reported in the paper and how they were run. (Example: We ran the NAS Parallel Benchmarks v3.3.1 on NERSC's Cori supercomputer with both Cray's version of MPICH 3.2.1 and with our SuperPGAS communication layer (v0.2), as described in the paper.). MathJax is enabled so you can enter LaTeX mathematical notation within \(...\) or \[...\].

In this article, we have run three types of experiments:
1) iperf for measuring bandwidth in 3 clouds: Amazon EC2 (us-east), Google (us-east), and HPCCloud (https://userinfo.surfsara.nl/systems/hpc-cloud);
The data artifacts can be found in the repository pointed at, for figures 4, 5, and 6.
The iperf version is 3.0.7 (Amazon), and 3.0.11 (Google and HPCCloud). All the experiment
parameters are logged by iperf in the output files that we give as artifacts.
2) HiBench v7.0 and TPC-DS (https://github.com/databricks/spark-sql-perf) 
experiments, emulating the A-H bandwidth setups from Ballani et al. [1].
The script used for emulation is released as code artifact. HiBench and TPC-DS are run
under Spark 2.4.0, which runs on Java 1.8.0_131.
3) HiBench v7.0 and TPC-DS (https://github.com/databricks/spark-sql-perf) 
experiments, emulating the token bucket policy and mechanisms identified at point 1).
The script used for emulation is released as code artifact. HiBench and TPC-DS are run
under Spark 2.4.0, which runs on Java 1.8.0_131.

most important parameters:
Spark configuration that works for nodes with 16 cores and 64GB memory, goes into spark-env.sh:
SPARK_EXECUTOR_CORES=4
SPARK_EXECUTOR_MEMORY=15g
SPARK_WORKER_INSTANCES=4
SPARK_WORKER_CORES=4
SPARK_WORKER_MEMORY=15g

HiBench, goes into hibench.conf:
# Mapper number in hadoop, partition number in Spark
hibench.default.map.parallelism         2048
# Reducer nubmer in hadoop, shuffle partition number in Spark
hibench.default.shuffle.parallelism     2048

Artifacts Evaluation — Describe if and how you:
(a) Performed verification and validation studies:
1) The Cloud measurements:
As we report in the paper, we have run our experiments over large periods of time (weeks),
to eliminate the effects of transient cloud behavior. Moreover, we run smaller scale experiments,
over different types of machines, to validate whether their behavior falls into the bounds discovered
with the longer term studies. Moreover, being able to implement an emulator that closely follows
the identified token bucket policies and mechanisms leads to the conclusion that what we have
measured is not random noise, but rather the intended behavior.
2) The big data measurements:
a) gigabit era: we have performed sufficient repetitions that enabled us to perform confidence interval
analysis, and to conclude that after sufficient experiments (30-50), the confidence intervals
are tight enough to fall within 10% error bounds.
b) post-gigabit era: we have performed sufficient repetitions to confirm that within a given
token bucket budget, most applications achieve tight confidence intervals, leading to the
conclusion that our experimentation is accurate and does not include (much) noise.

(b) Validated the accuracy and precision of timings:
We have used state-of-the-art benchmarks for both measuring network bandwidth, and also for
running big data applications - HiBench and TPC-DS. These are complex pieces of software,
and we rely on their ability to properly capture the behavior of a system. However, we are
encouraged by the fact that all three are community-driven, open-source approaches, that are widely respected and adopted.

(c) Used manufactured solutions or spectral properties:

(d) Quantified the sensitivity of your results to initial conditions and/or parameters of the computational environment:
Our study, as described in the paper, is exactly about the interaction between the variable
conditions of the underlying system (i.e., cloud) and the application (big data). To eliminate,
or minimize the effect of the transient system conditions, we run our workloads under emulation,
in an empty cluster, that does not share resources. We emulate only variable network conditions,
such that our results only describe the interaction of variable networks and big data applications.
In addition to running in emulation, in a non-shared cluster, we make sure that each run we show
is performed on fresh machines, without any warming-up effects, flushed caches etc. 

(e) Describe controls, statistics, or other steps taken to make the measurements and analyses robust to variability and unknowns in the system.
Since our study is exactly about the effects of performance variability on big data applications,
we actually compute confidence intervals for the median and the tail (90th percentile), and show
that with enough repetitions the confidence intervals fall within 10\% error bounds. We also show
when this is not the case (for networks with token bucket mechanisms for QoS) and give the reader
advice on how to overcome this. As suggested by the best practices for robust analysis
of computer performance, we estimated and analyzed nonparametetric (asymmetric) confidence
intervals for medians and 90th percentiles, which handle skew in the performance data  
and do make the assumption of normality in the studied distributions. 
To adequately characterize performance variability, we repeated our cloud experiments up to 50 times.
